# Supplementary material for: Percolation properties of the neutron population in nuclear reactors
Source: arXiv:2210.02413 source file (2022-10-05)
Supplement: Supplementary file 1 [file appendix_b.tex]

\section{Explicit form of the propagators in the two species model}
\label{app_b}
Setting $\Omega = 4 \beta \lambda_D + \lambda_D^2 + 2 \lambda_D r + r^2$, one has, 
\begin{eqnarray}
    \Sigma_{NN}(t,t') &=& \frac{e^{ \frac{1}{2} (r - \lambda_D)(t - t')  }}{\sqrt{\Omega}} \left\{  \sqrt{\Omega} \cosh\left(  \frac{1}{2} \sqrt{\Omega} (t - t') \right) \right. \nonumber\\
    & & \left.  + (r + \lambda_D) \sinh\left(  \frac{1}{2} \sqrt{\Omega} (t - t') \right)  \right\},
\end{eqnarray}

\begin{eqnarray}
    \Sigma_{MM}(t,t') &=& \frac{e^{ \frac{1}{2} (r - \lambda_D)(t - t')  }}{\sqrt{\Omega}} \left\{  \sqrt{\Omega} \cosh\left(  \frac{1}{2} \sqrt{\Omega} (t - t') \right) \right. \nonumber\\
    & & \left.  - (r + \lambda_D) \sinh\left(  \frac{1}{2} \sqrt{\Omega} (t - t') \right)  \right\},
\end{eqnarray}

\begin{equation}
        \Sigma_{NM}(t,t') = 2 \beta \frac{e^{ \frac{1}{2} (r - \lambda_D)(t - t')  }}{\sqrt{\Omega}} \sinh\left(  \frac{1}{2} \sqrt{\Omega} (t - t') \right),
\end{equation}

\begin{equation}
    \Sigma_{MN}(t,t') = 2 \lambda_D \frac{e^{ \frac{1}{2} (r - \lambda_D)(t - t')  }}{\sqrt{\Omega}} \sinh\left(  \frac{1}{2} \sqrt{\Omega} (t - t') \right) .
\end{equation}
